# Supplementary material for: Convex Optimization for Linear Query Processing under Approximate Differential Privacy
Source: arXiv:1602.04302 source file (2016-05-16)
Supplement: Supplementary file 1 [file appendix.tex]

\input{appsdp.tex}

\input{appdual.tex}

\input{appbound.tex}

\input{appadd.tex}

\input{appconv.tex}
